# Supplementary material for: Introduction to Quantum Error Correction and Fault Tolerance
Source: arXiv:2111.08894 source file (2023-01-06)
Supplement: Supplementary file 1 [file Appendix1_v3.tex]

\section{Density Matrices and the Wigner Function}
\label{app:Wigner}

The density matrix for a quantum system is defined by\footnote{The material in this appendix is based on the author's 2016 Les Houches Lectures \cite{GirvinLesHouches2016}.}
 \begin{equation}
 {\hat\rho}\equiv \sum_j |\psi_j\rangle p_j\langle \psi_j|
 \end{equation}
where where $p_j$ is the statistical probability that the system is found in state $|\psi_j\rangle$.
As we will see further below, this is a useful quantity because it provides all the information needed to calculate the expectation value of any quantum observable $\mathcal O$.
In thermal equilibrium, $|\psi_j\rangle$ is the $j$th energy eigenstate with eigenvalue $\epsilon_j$ and $p_j=\frac{1}{Z}e^{-\beta \epsilon_j}$ is the corresponding Boltzmann weight.  In this case the states are all naturally orthogonal, $\langle \psi_j|\psi_k\rangle = \delta_{jk}$.  It is important to note however that in general the only constraint on the probabilities is that they are non-negative and sum to unity.  Furthermore there is \emph{no} requirement that the states be orthogonal (or complete), only that they be normalized.

The expectation value of an observable ${\mathcal O}$ is given by
\begin{equation}
\langle\langle{\mathcal O}\rangle\rangle=\mathrm{Tr}\,{\mathcal O}{\hat\rho}
\end{equation}
where the double brackets indicate both quantum and statistical ensemble averages.  To prove this result, let us evaluate the trace in the complete orthonormal set of eigenstates of ${\mathcal O}$ obeying ${\mathcal O}|m\rangle=O_m|m\rangle$.  In this basis the observable has the representation
\begin{equation}
{\mathcal O}=\sum_m |m\rangle O_m\langle m|
\end{equation}
and thus we can write
\begin{eqnarray}
\mathrm{Tr}\,{\mathcal O}{\hat\rho} &=& \sum_m\langle m|{\mathcal O}{\hat\rho}|m\rangle\nonumber\\
&=&\sum_m O_m \sum_j \langle m|\psi_j\rangle p_j\langle \psi_j|m\rangle\nonumber\\
&=&\sum_j p_j \sum_m\langle\psi_j|m\rangle O_m \langle m|\psi_j\rangle \nonumber\\
&=&\sum_j p_j \langle\psi_j|{\mathcal O}|\psi_j\rangle \equiv
\langle\langle {\mathcal O}\rangle\rangle.
\end{eqnarray}
Notice the important fact that if $\mathcal{O}$ is the identity operator we obtain
\begin{equation}
\mathrm{Tr}\,{\hat\rho}=\sum_j p_j=1.
\end{equation}
This is true independent of whether or not the $\{\psi_j\}$ are orthogonal, so long as they are normalized.  Also notice another important property of the density matrix, it is Hermitian and for any state vector $|\Phi\rangle$ we have
\begin{eqnarray}
\langle\Phi|{\hat\rho}|\Phi\rangle=\sum_j p_j \langle\Phi|\psi_j\rangle\langle\psi_j|\Phi\rangle \ge 0.
\end{eqnarray}
Hence every density matrix is positive semi-definite (i.e., its eigenvalues are real and non-negative) and has unit trace (i.e., the sum of the eigenvalues is unity).   For a single qubit, the density matrix is a $2\times 2$ Hermitian matrix.  Since the Identity and the three Pauli matrices span the space of such matrices, the most general density matrix for a single qubit is
\begin{equation}
{\hat\rho}=\frac{1}{2}\left[\hat I+\vec m\cdot\vec \sigma\right].
\end{equation}
To guarantee that ${\hat\rho}$ is positive semi-definite, the `polarization vector' $\vec m = (m_x,m_y,m_z)$ must have length $|\vec m|\le 1$.
For $|\vec m|=1$, we have a pure state and $\vec m$ is the point on the Bloch sphere describing the state $|\vec m\rangle$.  If $\vec m$ lies in the interior of the Bloch sphere, we have an impure state that is an incoherent mixture of $|{\hat m}\rangle$
and $|-{\hat m}\rangle$, where ${\hat m}$ is the unit vector parallel to $\vec m$ and
\begin{equation}
{\hat\rho}=\Lambda|{+\hat m}\rangle\langle{+\hat m}| +(1-\Lambda)|{-\hat m}\rangle\langle{-\hat m}|,
\end{equation}
with $\Lambda\equiv \langle\vec\sigma\cdot\hat m\rangle$ being the magnitude of the polarization.
A convenient property of this representation of the density matrix in terms of the polarization vector is that
\begin{equation}
\langle \vec\sigma\rangle = \vec m.
\label{eq:rhopolarization}
\end{equation}
For $|\vec m|=0$ we have $\Lambda$=0 and thus a completely mixed state,
\begin{equation}
{\hat\rho}=\frac{1}{2}\left(\begin{array}{cc}1&0\\0&1\end{array}\right).
\end{equation}

Since ${\hat\rho}$ is Hermitian, it can always be diagonalized.  A pure state has density matrix with rank 1 (i.e., only one non-zero eigenvalue which must necessarily equal $+1$.  In this state there is no uncertainty about which state the system is in.  Since a pure state density matrix is a projector, we have ${\hat\rho}^2={\hat\rho}$ for pure states.  We can define a formal measure of the purity of a state via the trace of ${\hat\rho}^2$
\begin{equation}
\frac{1}{d} \le \mathrm{Tr}\, {\hat\rho}^2\le 1,
\end{equation}
where $d$ is the dimension of the Hilbert space.
Here we are slipping into a sloppy but standard usage of calling a density matrix a state.  It is not a state in the Hilbert space but rather a description of the statistical distribution states in the Hilbert space.

\begin{mdframed}
	\begin{Exercise}
Derive eqn~(\ref{eq:rhopolarization}).  Use the fact that the Pauli matrices are traceless and square to the Identity.  
\end{Exercise}
\end{mdframed}

After the above general introduction, we now specialize to the case of a continuous-variable system, namely a single-particle moving in one spatial dimension.  A useful example is the harmonic oscillator model which might represent a mechanical oscillator or the electromagnetic oscillations of a particular mode of a microwave or optical cavity.  Our first task is to understand the relationship between the quantum density matrix and the classical phase space distribution.

In classical statistical mechanics we are used to thinking about the probability density $P(x,p)$ of finding a particle at a certain point in phase space.  For example, in thermal equilibrium the phase space distribution is simply
  \begin{equation}
  P(x,p)\frac{dxdp}{2\pi\hbar}=\frac{1}{Z}e^{-\beta H(x,p)}\frac{dxdp}{2\pi\hbar},
  \end{equation}
  where the partition function is given by
  \begin{equation}
 Z=\int\int \frac{dxdp}{2\pi\hbar} e^{-\beta H(x,p)},
  \end{equation}
  and where for convenience (and planning ahead for the quantum case) we have made the phase space measure dimensionless by inserting the factor of Planck's constant.
The marginal distributions for position and momentum are found by
\begin{eqnarray}
{\hat\rho}_1(x)&=&\frac{1}{2\pi\hbar}\int_{-\infty}^{+\infty}dp\,P(x,p)\label{eq:margx0}\\
{\hat\rho}_2(p)&=&\frac{1}{2\pi\hbar}\int_{-\infty}^{+\infty}dx\,P(x,p).\label{eq:margp0}
\end{eqnarray}

 Things are more complex in quantum mechanics because the observables $\hat x$ and $\hat p$ do not commute and hence cannot be simultaneously measured because of Heisenberg uncertainty. To try to make contact with the classical phase space distribution it is useful to study the quantum density matrix in the position representation given by
\begin{equation}
{\hat\rho}(x,x')=\langle x|{\hat\rho}|x'\rangle = \sum_j p_j \psi_j(x)\psi_j^*(x'),
\end{equation}
where the wave functions are given by $\psi_j(x)=\langle x|\psi_j\rangle$.
 It is clear from the Born rule that the marginal distribution for position can be found from the diagonal element of the density matrix
 \begin{equation}
  {\hat\rho}_1(x)={\hat\rho}(x,x)=\sum_j p_j |\psi_j(x)|^2.
 \label{eq:margx}
  \end{equation}
 Likewise the marginal distribution for momentum is given by the diagonal element of the density matrix in the momentum representation
 \begin{equation}
 {\hat\rho}_2(p)=\langle p|{\hat\rho}|p\rangle.
 \end{equation}
 We can relate this to the position representation by inserting resolutions of the identity in terms of complete sets of position eigenstates\footnote{Note that we are using unnormalized momentum eigenstates $\langle x|p\rangle = e^{ipx/\hbar}$.  Correspondingly we are not using a factor of the system size $L$ in the integration measure (`density of states in k space') for momentum.}
 \begin{eqnarray}
 \tilde{\hat\rho}(p,p') &=& \frac{1}{2\pi\hbar}\int_{-\infty}^{+\infty} dxdx'\, \langle p|x\rangle\langle x|{\hat\rho}|x'\rangle\langle x'|p'\rangle\nonumber\\
 &=& \frac{1}{2\pi\hbar}\int_{-\infty}^{+\infty} dxdx'\, e^{-ipx/\hbar}{\hat\rho}(x,x')e^{+ip'x'/\hbar}.
 \end{eqnarray}
 Thus the momentum representation of the density matrix is given by the Fourier transform of the position representation.  We see also
 that the marginal distribution for the momentum involves the off-diagonal elements of the real-space density matrix in an essential way
 \begin{equation}
 {\hat\rho}_2(p) = \frac{1}{2\pi\hbar}\int_{-\infty}^{+\infty} dxdx' e^{-ip(x-x')/\hbar}{\hat\rho}(x,x').
 \end{equation}
 For later purposes it will be convenient to define `center of mass' and `relative' coordinates
 $y=\frac{x+x'}{2}$ and $\xi=x-x'$ and reexpress this integral as
  \begin{equation}
 {\hat\rho}_2(p) =\frac{1}{2\pi\hbar} \int_{-\infty}^{+\infty} dy\int_{-\infty}^{+\infty}d\xi\, e^{-ip\xi/\hbar}{\hat\rho}(y+\xi/2,y-\xi/2).
 \label{eq:margp}
 \end{equation}

 Very early in the history of quantum mechanics, Wigner noticed from the above expression that one could write down a quantity which is a natural extension of the phase space density.  The so-called Wigner `quasi-probability distribution' is defined by
  \begin{equation}
 W(x,p)\equiv\frac{1}{2\pi\hbar} \int_{-\infty}^{+\infty}d\xi\, e^{-ip\xi/\hbar}{\hat\rho}(x+\xi/2,x-\xi/2).
 \label{eq:Wignerdef}
 \end{equation}
 Using this, eqn~(\ref{eq:margp}) becomes (changing the dummy variable $y$ back to $x$ for notational clarity)
\begin{equation}
 {\hat\rho}_2(p) = \int_{-\infty}^{+\infty} dx\, W(x,p).
 \label{eq:margp2}
 \end{equation}
 Similarly, by using eqn~(\ref{eq:Wignerdef}), we can write eqn~(\ref{eq:margx}) as
 \begin{equation}
 {\hat\rho}_1(x)=\int_{-\infty}^{+\infty} dp\, W(x,p).
 \label{eq:margx2}
 \end{equation}
 These equations are analogous to eqns~(\ref{eq:margx0},\ref{eq:margp0}) and show that the Wigner distribution is analogous to the classical phase space density $P(x,p)$.  However the fact that position and momentum do not commute turns out to mean that the Wigner distribution need not be positive.  In fact, in quantum optics one often takes the defining characteristic of non-classical states of light to be that they have Wigner distributions which are negative in some regions of phase space.

 The Wigner function is extremely useful in quantum optics because, like the density matrix, it contains complete information about the quantum state of an electromagnetic oscillator mode, but (at least in circuit QED) is much easier to measure.   Through a remarkable mathematical identity \cite{Davidovich1,HarocheRaimondcQEDBook} we can relate the Wigner function to the expectation value of the photon number parity, something that can be measured \cite{BertetWignerPhysRevLett.89.200402} and is especially easy to measure \cite{Vlastakisbigcat} in the strong-coupling regime of circuit QED (a regime not easy to reach in ordinary quantum optics).

 We are used to thinking of the photon number parity operator in its second quantized form
 \begin{equation}
 \hat\Pi=e^{i\pi a^\dagger a}
 \end{equation}
in which its effect on photon Fock states is clear
\begin{equation}
\hat\Pi|n\rangle = (-1)^n|n\rangle,
\end{equation}
and indeed it is in this form that it is easiest to understand how to realize the operation experimentally using time evolution under the cQED qubit-cavity coupling  $\chi \sigma^z a^\dagger a$ in the strong-dispersive limit of large $\chi$ relative to dissipation.  However because the Wigner function has been defined in a first quantization representation in terms of wave functions, it is better here to think about the parity operator in its first-quantized form.  Recalling that the wave functions of the simple harmonic oscillator energy eigenstates alternate in spatial reflection parity as one moves up the ladder, it is clear that photon number parity and spatial reflection parity are one and the same.  That is, if $|x\rangle$ is a position eigensate
\begin{equation}
\hat\Pi|x\rangle =|-x\rangle,
\end{equation}
or equivalently in terms of the wave function
\begin{equation}
\hat\Pi \psi(x) = \langle x|\hat\Pi|\psi\rangle = \psi (-x).
\end{equation}
To further cement the connection, we note that since the position operator is linear in the ladder operators, it is straightforward to verify from the second-quantized representations that
\begin{equation}
\hat\Pi\hat x= - \hat x \hat \Pi.
\end{equation}

We now want to show that we can measure the Wigner function $W(X,P)$ by the following simple and direct recipe \cite{Davidovich1}:  (1) displace the oscillator in phase space so that the point $(X,P)$ moves to the origin; (2)  then measure the expectation value of the photon number parity
\begin{equation}
W(X,P)=\frac{1}{\pi\hbar}\mathrm{Tr}\,\left\{{\mathcal D}(-X,-P){\hat\rho} {\mathcal D}^\dagger(-X,-P) \hat \Pi\right\},
\label{eq:dispP}
\end{equation}
where $\mathcal D$ is the displacement operator.
Related methods in which one measures not the parity but the full photon number distribution of the displaced state can in principle yield even more robust results in the presence of measurement noise \cite{LiangDisplacedNumberSampling}.

%\added{CHECK FACTOR OF 2 IN THE ABOVE}

Typically in experiment one would make a single `straight-line' displacement. Taking advantage of the fact that $\hat p$ is the generator of displacements in position and $\hat x$ is the generator of displacements in momentum, the `straight-line' displacement operator is given by
\begin{equation}
{\mathcal D}(-X,-P) = e^{-\frac{i}{\hbar}(P\hat x-X\hat p)}.
\label{eq:straightlinedisp}
\end{equation}
In experiment, this displacement operation is readily carried out by simply applying a pulse at the cavity resonance frequency with appropriately chosen amplitude, duration and phase.  In the frame rotating at the cavity frequency the drive corresponds to the following term in the Hamiltonian
\begin{equation}
V(t) = i[\epsilon(t)a^\dagger - \epsilon^*(t) a]
\label{eq:cavitydisplacement}
\end{equation}
where $\epsilon(t)$ is a complex function of time describing the two quadratures of the drive pulse.  The Heisenberg equation of motion
\begin{equation}
\frac{d}{dt}a=i[V(t),a]=\epsilon(t),
\end{equation}
has solution
\begin{equation}
a(t) = a(0) + \int_{-\infty}^t d\tau\, \epsilon(\tau),
\end{equation}
showing that the cavity is simply displaced in phase space by the drive.
  For the `straight-line' displacement discussed above, $\epsilon(t)$ has fixed phase and only the magnitude varies with time.

\begin{mdframed}[style=exampledefault]
\begin{Exercise}
Find an expression for $\epsilon(t)$ such that time evolution under the drive in eqn~(\ref{eq:cavitydisplacement}) will reproduce eqn~(\ref{eq:straightlinedisp}).  Ignore cavity damping (an assumption which is valid if the pulse duration is short enough).
\end{Exercise}
\end{mdframed}

For theoretical convenience in the present calculation, we will carry out the displacement in two steps by using the Feynman disentangling theorem
\begin{equation}
e^{\hat A +\hat B}=e^{\hat A}e^{\hat B}e^{\frac{1}{2}[\hat B,\hat A]}
\end{equation}
(which is valid if $[\hat B,\hat A]$ itself commutes with both $\hat A$ and $\hat B$) to write
\begin{equation}
{\mathcal D}(-X,-P)=e^{i\theta}{\mathcal D}(0,-P){\mathcal D}(-X,0)=e^{i\theta}e^{-\frac{i}{\hbar}P\hat x}e^{+\frac{i}{\hbar}X\hat p},
\end{equation}
where $\theta\equiv {\frac{i}{2\hbar}XP}$.
This form of the expression represents a move of the phase space point $(X,P)$ to the origin by first displacing the system in position by $-X$ and then in momentum by $-P$.  This yields the same final state as the straightline displacement except for an overall phase $\theta$ which arises from the fact that displacements in phase space do not commute.  For present purposes this overall phase drops out and we will ignore it henceforth.

Under this pair of transformations the wave function becomes
\begin{equation}
\psi(x)\rightarrow \psi(x+X)\rightarrow e^{-iPx/\hbar}\psi(x+X).
\end{equation}
More formally, we have two results which will be useful in evaluating eqn~(\ref{eq:dispP})
\begin{eqnarray}
\langle \xi|{\mathcal D}(0,-P){\mathcal D}(-X,0)|\psi \rangle &=& e^{-iP\xi/\hbar}\psi(\xi+X)\\
\langle \psi|{\mathcal D}^\dagger(-X,0){\mathcal D}^\dagger(0,-P)|\xi\rangle&=&e^{+iP\xi/\hbar}\psi^*(\xi+X).
\end{eqnarray}
Taking the trace in eqn~(\ref{eq:dispP}) in the position basis yields
\begin{eqnarray}
W(X,P)&=&\frac{1}{\pi\hbar}\sum_j p_j\int_{-\infty}^{+\infty}d\xi\, \langle \xi|{\mathcal D}(-X,-P)|\psi_j\rangle  \langle \psi_j| {\mathcal D}^\dagger(-X,-P) \hat \Pi|\xi\rangle\nonumber\\
&=&\frac{1}{\pi\hbar}\sum_j p_j\int_{-\infty}^{+\infty}d\xi\, \langle \xi|{\mathcal D}(-X,-P)|\psi_j\rangle  \langle \psi_j| {\mathcal D}^\dagger(-X,-P) |-\xi\rangle\nonumber\\
&=&\frac{1}{\pi\hbar}\sum_j p_j\int_{-\infty}^{+\infty}d\xi\, e^{-iP2\xi/\hbar}\psi_j(\xi+X)\psi_j^*(-\xi+X)\nonumber\\
&=&\frac{1}{2\pi\hbar}\sum_j p_j\int_{-\infty}^{+\infty}d\xi\, e^{-iP\xi/\hbar}\psi_j(X+\xi/2)\psi_j^*(X-\xi/2),
\label{eq:dispP2}
\end{eqnarray}
which proves that the displaced parity is indeed precisely the Wigner function.
